# Supplementary material for: Local Area Transform for Cross-Modality Correspondence Matching and Deep Scene Recognition
Source: arXiv:1901.00927 source file (2019-01-03)
Supplement: Supplementary file 1 [file SupplementaryMaterial.tex]

% last updated in April 2002 by Antje Endemann
% Based on CVPR 07 and LNCS, with modifications by DAF, AZ and elle, 2008 and AA, 2010, and CC, 2011; TT, 2014

%\documentclass[runningheads]{llncs}
\usepackage{graphicx}
\usepackage{multirow}
\usepackage{subfigure}
\usepackage{tabulary}
\usepackage{setspace}
\usepackage{array}
\usepackage{longtable}
\usepackage{makecell}

\usepackage{amsmath,amssymb} % define this before the line numbering.
\usepackage{ruler}
\usepackage{color}
\usepackage[width=122mm,left=12mm,paperwidth=146mm,height=193mm,top=12mm,paperheight=217mm]{geometry}
\begin{document}
% \renewcommand\thelinenumber{\color[rgb]{0.2,0.5,0.8}\normalfont\sffamily\scriptsize\arabic{linenumber}\color[rgb]{0,0,0}}
% \renewcommand\makeLineNumber {\hss\thelinenumber\ \hspace{6mm} \rlap{\hskip\textwidth\ \hspace{6.5mm}\thelinenumber}}
% \linenumbers
\newcolumntype{C}[1]{>{\centering\let\newline\\\arraybackslash\hspace{0pt}}m{#1}}
\pagestyle{headings}
\mainmatter
\def\ECCV14SubNumber{1941}  % Insert your submission number here

\title{Supplementary Material} % Replace with your title

\titlerunning{CVPR15 submission ID \ECCV14SubNumber}

\authorrunning{CVPR15 submission ID \ECCV14SubNumber}

\author{Anonymous CVPR submission}
\institute{Paper ID \ECCV14SubNumber}

\maketitle

\vspace{10pt}
\noindent This supplementary material includes further results which are not included in the submitted paper listed as follows. Importantly, note that the supplementary materials are not necessary to understand the submitted paper.

\begin{itemize}
\item Original test color images used in Section 4.1 \vspace{5pt}
\item Robustness comparison of GW, HM, LC, RT, and LAT for nonlinear intensity deformations (related to Section 4.1 in the submitted paper) \vspace{5pt}
\item Supplementary results for cross-spectral template matching (related to Section 4.2 in the submitted paper) \vspace{5pt}
\item Supplementary results for robust stereo matching (related to Section 4.3 in the submitted paper) \vspace{5pt}
\end{itemize}

\section{Original test color images used in Section 4 of the Submitted Paper}

Fig. 1 presents the original test color images used in Section 4 of the submitted paper.

\begin{figure}[!h]
\renewcommand{\thesubfigure}{}
\centering{
\includegraphics[width=0.24\linewidth]{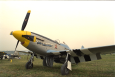}
\includegraphics[width=0.24\linewidth]{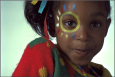}
\includegraphics[width=0.24\linewidth]{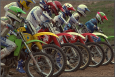}
\includegraphics[width=0.24\linewidth]{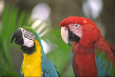}
\linebreak
\linebreak
\includegraphics[width=0.24\linewidth]{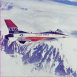}
\includegraphics[width=0.24\linewidth]{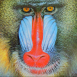}
\includegraphics[width=0.24\linewidth]{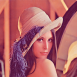}
\includegraphics[width=0.24\linewidth]{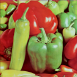}
}
\vspace{-5pt}
\caption{The original test color images used in Section 4 of the submitted paper}
\end{figure}

\section{Robustness comparison for nonlinear intensity deformations}

Figs. 2-4 show the examples of robustness comparison for nonlinear intensity deformations with Mustang, Airplane, and Peppers, respectively. Note that, for all test images and deformations, the tendency of results are similar.

\begin{figure}[!h]
\renewcommand{\thesubfigure}{}
\centering{
\subfigure[(a) ORG]{\includegraphics[width=0.18\linewidth]{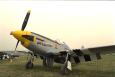}
\includegraphics[width=0.18\linewidth]{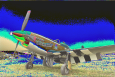}
\includegraphics[width=0.18\linewidth]{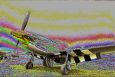}
\includegraphics[width=0.18\linewidth]{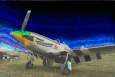}
\includegraphics[width=0.18\linewidth]{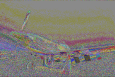}}
\subfigure[(b) GW]{\includegraphics[width=0.18\linewidth]{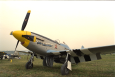}
\includegraphics[width=0.18\linewidth]{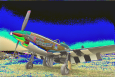}
\includegraphics[width=0.18\linewidth]{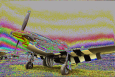}
\includegraphics[width=0.18\linewidth]{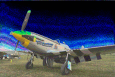}
\includegraphics[width=0.18\linewidth]{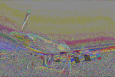}}
\subfigure[(c) HM]{\includegraphics[width=0.18\linewidth]{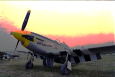}
\includegraphics[width=0.18\linewidth]{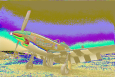}
\includegraphics[width=0.18\linewidth]{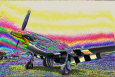}
\includegraphics[width=0.18\linewidth]{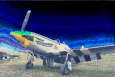}
\includegraphics[width=0.18\linewidth]{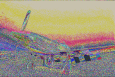}}
\subfigure[(d) LC]{\includegraphics[width=0.18\linewidth]{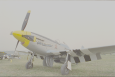}
\includegraphics[width=0.18\linewidth]{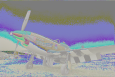}
\includegraphics[width=0.18\linewidth]{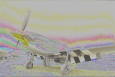}
\includegraphics[width=0.18\linewidth]{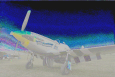}
\includegraphics[width=0.18\linewidth]{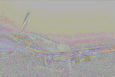}}
\subfigure[(e) RT]{\includegraphics[width=0.18\linewidth]{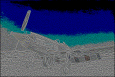}
\includegraphics[width=0.18\linewidth]{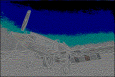}
\includegraphics[width=0.18\linewidth]{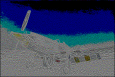}
\includegraphics[width=0.18\linewidth]{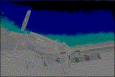}
\includegraphics[width=0.18\linewidth]{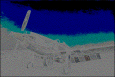}}
\subfigure[(f) LAT]{\includegraphics[width=0.18\linewidth]{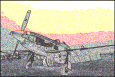}
\includegraphics[width=0.18\linewidth]{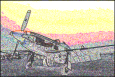}
\includegraphics[width=0.18\linewidth]{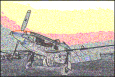}
\includegraphics[width=0.18\linewidth]{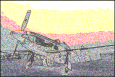}
\includegraphics[width=0.18\linewidth]{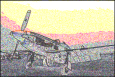}}}
\vspace{-5pt}
\caption{The robustness comparison for nonlinear intensity deformations for Mustang. For each sub-figure, from left to right, figures are non-deformed image, deformed images by piecewise-linear mapping, deformed images by piecewise-quadratic mapping, deformed images by random mapping with Gaussian distribution, deformed images by random mapping with uniform distribution. The figures are best viewed in color.}
\end{figure}

\begin{figure}[!h]
\renewcommand{\thesubfigure}{}
\centering{
\subfigure[(a) ORG]{\includegraphics[width=0.18\linewidth]{Figures_Supplementary/Fig1_Airplane.png}
\includegraphics[width=0.18\linewidth]{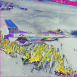}
\includegraphics[width=0.18\linewidth]{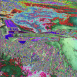}
\includegraphics[width=0.18\linewidth]{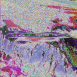}
\includegraphics[width=0.18\linewidth]{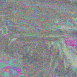}}
\subfigure[(b) GW]{\includegraphics[width=0.18\linewidth]{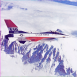}
\includegraphics[width=0.18\linewidth]{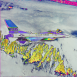}
\includegraphics[width=0.18\linewidth]{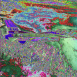}
\includegraphics[width=0.18\linewidth]{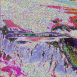}
\includegraphics[width=0.18\linewidth]{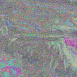}}
\subfigure[(c) HM]{\includegraphics[width=0.18\linewidth]{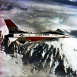}
\includegraphics[width=0.18\linewidth]{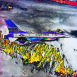}
\includegraphics[width=0.18\linewidth]{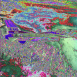}
\includegraphics[width=0.18\linewidth]{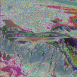}
\includegraphics[width=0.18\linewidth]{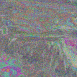}}
\subfigure[(d) LC]{\includegraphics[width=0.18\linewidth]{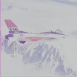}
\includegraphics[width=0.18\linewidth]{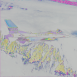}
\includegraphics[width=0.18\linewidth]{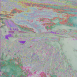}
\includegraphics[width=0.18\linewidth]{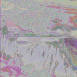}
\includegraphics[width=0.18\linewidth]{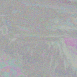}}
\subfigure[(e) RT]{\includegraphics[width=0.18\linewidth]{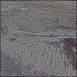}
\includegraphics[width=0.18\linewidth]{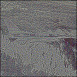}
\includegraphics[width=0.18\linewidth]{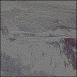}
\includegraphics[width=0.18\linewidth]{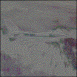}
\includegraphics[width=0.18\linewidth]{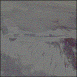}}
\subfigure[(f) LAT]{\includegraphics[width=0.18\linewidth]{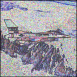}
\includegraphics[width=0.18\linewidth]{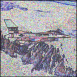}
\includegraphics[width=0.18\linewidth]{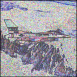}
\includegraphics[width=0.18\linewidth]{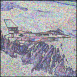}
\includegraphics[width=0.18\linewidth]{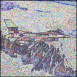}}}
\vspace{-5pt}
\caption{The robustness comparison for nonlinear intensity deformations for Airplane. For each sub-figure, from left to right, figures are non-deformed image, deformed images by piecewise-linear mapping, deformed images by piecewise-quadratic mapping, deformed images by random mapping with Gaussian distribution, deformed images by random mapping with uniform distribution. The figures are best viewed in color.}
\end{figure}

\begin{figure}[!h]
\renewcommand{\thesubfigure}{}
\centering{
\subfigure[(a) ORG]{\includegraphics[width=0.18\linewidth]{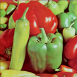}
\includegraphics[width=0.18\linewidth]{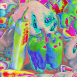}
\includegraphics[width=0.18\linewidth]{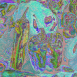}
\includegraphics[width=0.18\linewidth]{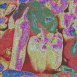}
\includegraphics[width=0.18\linewidth]{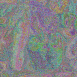}}
\subfigure[(b) GW]{\includegraphics[width=0.18\linewidth]{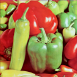}
\includegraphics[width=0.18\linewidth]{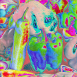}
\includegraphics[width=0.18\linewidth]{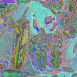}
\includegraphics[width=0.18\linewidth]{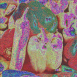}
\includegraphics[width=0.18\linewidth]{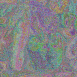}}
\subfigure[(c) HM]{\includegraphics[width=0.18\linewidth]{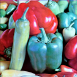}
\includegraphics[width=0.18\linewidth]{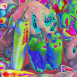}
\includegraphics[width=0.18\linewidth]{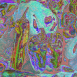}
\includegraphics[width=0.18\linewidth]{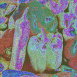}
\includegraphics[width=0.18\linewidth]{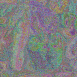}}
\subfigure[(d) LC]{\includegraphics[width=0.18\linewidth]{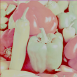}
\includegraphics[width=0.18\linewidth]{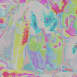}
\includegraphics[width=0.18\linewidth]{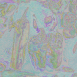}
\includegraphics[width=0.18\linewidth]{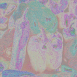}
\includegraphics[width=0.18\linewidth]{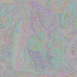}}
\subfigure[(e) RT]{\includegraphics[width=0.18\linewidth]{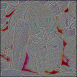}
\includegraphics[width=0.18\linewidth]{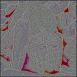}
\includegraphics[width=0.18\linewidth]{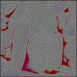}
\includegraphics[width=0.18\linewidth]{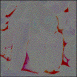}
\includegraphics[width=0.18\linewidth]{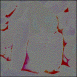}}
\subfigure[(f) LAT]{\includegraphics[width=0.18\linewidth]{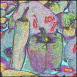}
\includegraphics[width=0.18\linewidth]{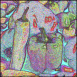}
\includegraphics[width=0.18\linewidth]{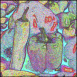}
\includegraphics[width=0.18\linewidth]{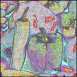}
\includegraphics[width=0.18\linewidth]{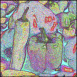}}}
\vspace{-5pt}
\caption{The robustness comparison for nonlinear intensity deformations for Pepper. For each sub-figure, from left to right, figures are non-deformed image, deformed images by piecewise-linear mapping, deformed images by piecewise-quadratic mapping, deformed images by random mapping with Gaussian distribution, deformed images by random mapping with uniform distribution. The figures are best viewed in color.}
\end{figure}

\clearpage

\clearpage
\section{Supplementary results for robust stereo matching}
\vspace{-10pt}
Figs. 7-9 present supplementary results for robust stereo matching providing better understandable visualization.
\vspace{-10pt}

\begin{figure}[!h]
\renewcommand{\thesubfigure}{}
\centering{
\subfigure[(a) ORG]{\includegraphics[width=0.20\linewidth]{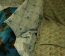}
\includegraphics[width=0.20\linewidth]{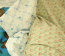}
\includegraphics[width=0.20\linewidth]{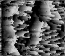}}
\subfigure[(a) GW]{\includegraphics[width=0.20\linewidth]{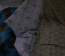}
\includegraphics[width=0.20\linewidth]{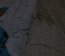}
\includegraphics[width=0.20\linewidth]{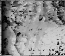}}
\subfigure[(a) HM]{\includegraphics[width=0.20\linewidth]{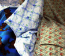}
\includegraphics[width=0.20\linewidth]{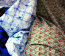}
\includegraphics[width=0.20\linewidth]{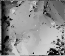}}
\subfigure[(a) LC]{\includegraphics[width=0.20\linewidth]{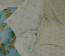}
\includegraphics[width=0.20\linewidth]{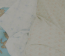}
\includegraphics[width=0.20\linewidth]{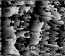}}
\subfigure[(a) RT]{\includegraphics[width=0.20\linewidth]{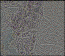}
\includegraphics[width=0.20\linewidth]{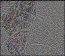}
\includegraphics[width=0.20\linewidth]{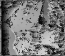}}
\subfigure[(a) LAT]{\includegraphics[width=0.20\linewidth]{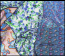}
\includegraphics[width=0.20\linewidth]{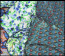}
\includegraphics[width=0.20\linewidth]{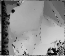}}

}
\vspace{-5pt}
\caption{Examples of robust stereo matching for Cloth2. For better understandable visualization (corresponding to Fig. 3(b) in the submitted paper), transformed images and disparity map are given. The figures are best viewed in color.}
\end{figure}

\begin{figure}[!h]
\renewcommand{\thesubfigure}{}
\centering{
\subfigure[(a) ORG]{\includegraphics[width=0.20\linewidth]{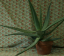}
\includegraphics[width=0.20\linewidth]{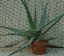}
\includegraphics[width=0.20\linewidth]{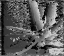}}
\subfigure[(a) GW]{\includegraphics[width=0.20\linewidth]{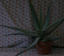}
\includegraphics[width=0.20\linewidth]{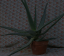}
\includegraphics[width=0.20\linewidth]{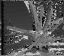}}
\subfigure[(a) HM]{\includegraphics[width=0.20\linewidth]{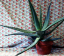}
\includegraphics[width=0.20\linewidth]{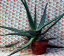}
\includegraphics[width=0.20\linewidth]{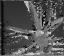}}
\subfigure[(a) LC]{\includegraphics[width=0.20\linewidth]{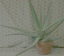}
\includegraphics[width=0.20\linewidth]{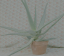}
\includegraphics[width=0.20\linewidth]{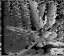}}
\subfigure[(a) RT]{\includegraphics[width=0.20\linewidth]{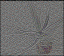}
\includegraphics[width=0.20\linewidth]{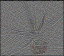}
\includegraphics[width=0.20\linewidth]{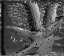}}
\subfigure[(a) LAT]{\includegraphics[width=0.20\linewidth]{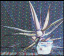}
\includegraphics[width=0.20\linewidth]{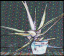}
\includegraphics[width=0.20\linewidth]{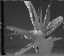}}

}
\vspace{-5pt}
\caption{Examples of robust stereo matching for Aloe. For better understandable visualization (corresponding to Fig. 3(c) in the submitted paper), transformed images and disparity map are given. The figures are best viewed in color.}
\end{figure}

\end{document}
